# Supplementary material for: Channel Impulse Response-based Physical Layer Authentication in a Diffusion-based Molecular Communication System
Source: arXiv:1907.08041 source file (2019-07-18)
Supplement: Supplementary file 1 [file appendix.tex]

\section{Least-Squares based DbMC Channel Impulse Response Estimation \cite{Jitendra:COMSNETS:2010}, \cite{} }
\label{app:cir_est}

The symbols $b[k]$ sent by the nano transmitter and the signal $r[k]$ received by the nano receiver are related as: $r[k]=b[k]\ast h[k]+w[k]=\sum_{l=0}^{L} h[l]b[k-l]+w[k]$. This work considers a training-based, least-squares approach to THz CIR estimation. Let $\{b[k]\}_{k=k_1}^{k=k_m}$ denote the training symbols. Define: $\mathbf{h}=[h[0],...,h[L]]^T$; basically $\mathbf{h}$ contains the $L+1$ taps of the CIR. Furthermore, let $\mathbf{r}=[r[k_1+L],r[k_1+L+1],...,r[k_m]]^T$, $\mathbf{w}=[w[k_1+L],w[k_1+L+1],...,w[k_m]]^T$. Then: 
\begin{equation}
{\mathbf{B}} = 
 \begin{pmatrix}
  b[k_1+L] & b[k_1+L-1] & \cdots & b[k_1] \\
  b[k_1+L+1] & b[k_1+L] & \cdots & b[k_1+1] \\
  \vdots  & \vdots  & \ddots & \vdots  \\
  b[k_m] & b[k_m-1] & \cdots & b[k_m-L] 
 \end{pmatrix}
\end{equation}

Then, the received signal at the nano receiver can be compactly written in matrix-vector form as:
\begin{equation}
{\mathbf{r}} = {\mathbf{B}}{\mathbf{h}} + {\mathbf{w}}
\end{equation}

Finally, the least-squares (LS) based estimate of the THz CIR is given as:
\begin{equation}
\label{eq:lsest}
\hat{\mathbf{h}} = ({\mathbf{B}^H}{\mathbf{B}})^{-1}{\mathbf{B}^H}{\mathbf{r}} 
\end{equation}

Specifically, $\hat{\mathbf{h}} \sim \mathcal{N}({\mathbf{h}},{\mathbf{\Sigma}_h})$ where ${\mathbf{\Sigma}_h} = \sigma^2({\mathbf{B}^H}{\mathbf{B}})^{-1}$. 

It is worth mentioning that the proposed least-squares based solution exists only when $\mathbf{B}$ is a full column-rank matrix. In other words, the length of training data should be: $k_m-k_1 \geq 2L$.
